# Supplementary material for: The maximum matching extendability and factor-criticality of 1-planar graphs
Source: arXiv:2205.12122 ancillary file (2022-05-24)
Supplement: Supplementary file 1 [file The_instruction_for_computer_programs.pdf]

# The instruction for computer programs

We can validate the five examples that we have given in the main text by using C++ programs.

The input data of the program is the adjacency list of a graph  $G$  with  $p$  vertices and the maximum degree  $d$ , which can be constructed as a  $p \times d$  array: First we label all the vertices in  $G$  by numbers from 1 to  $p$ , then the  $i$ th row represents all vertices adjacent to  $i$ -th vertex,  $1 \leq i \leq p$ . For those vertices that do not reach the maximum degree, we add a virtual adjacent vertex, labelled  $p + 1$  at the end of this row. This way we have got the five adjacency lists with names: graph\_5.txt, graph\_6.txt, graph\_7.txt, graph\_8(a).txt, graph\_8(b).txt corresponding to graphs in Figures 5, 6, 7, 8(a), 8(b) respectively.

## 1 Validation of Figure 5

First we verify that the graph in Fig. 5 in the main text is 4-extendable. We label each vertex of Fig. 5 as follows.

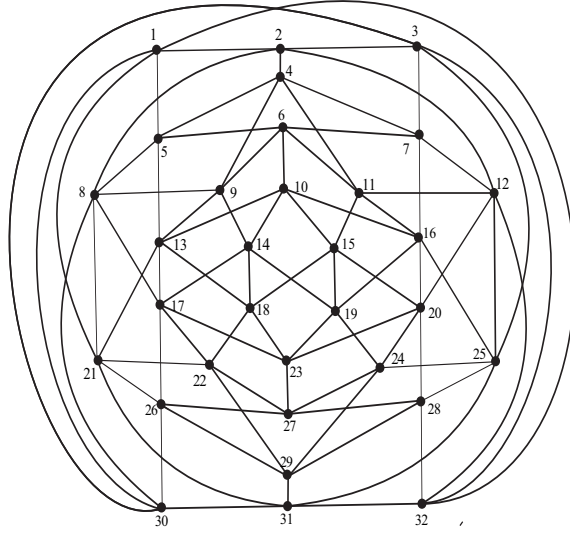

Fig. 5. A 4-extendable 1-planar graph.

Then run the program “matching\_extendability.cpp”. In the program, the txt file “graph\_5.txt” is the input data which is adjacency list of the graph, and the “extendable\_edges\_5.txt” is the output file which stores all 4-matchings in this graph. If there exists a running result 0, then the 4-matching cannot extend to a perfect matching; otherwise, it can be extended to a perfect matching. In the results we can see that none of 4-matchings results in 0. So the graph is 4-extendable.

## 2 Validation of Fig. 6

In this section, we check that the graph in Fig. 6 is 6-factor-critical in the main text. First we label each vertex of Fig. 6 as follows. Then we obtain its adjacency list (see graph\_6.txt)

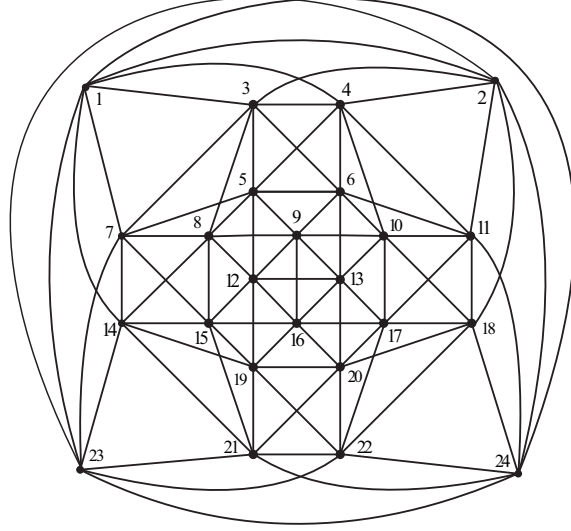

Fig. 6. A 6-factor-critical 1-planar graph.

Then run the program “factor\_critical.cpp”. In the program, the txt file “graph\_6.txt” is the input data which is adjacency list of the graph, and the “factor.txt” is the output file which stores all the cases of selected six vertices in this graph. If a running result is 0, then the graph is not 6-factor-critical; otherwise, it is 6-factor-critical. In the results we can see that none of the selected six vertices results in 0. So the graph is 6-factor-critical.

## 3 Validation of Figs. 7, 8(a) and (b)

Similar to Fig. 6 we can confirm that the graphs in Fig. 7 and Figs. 8(a) and (b) are 5-, 4- and 5-factor-critical by using the same program “factor\_critical.cpp”. First we also label the vertices of such graphs as follows.

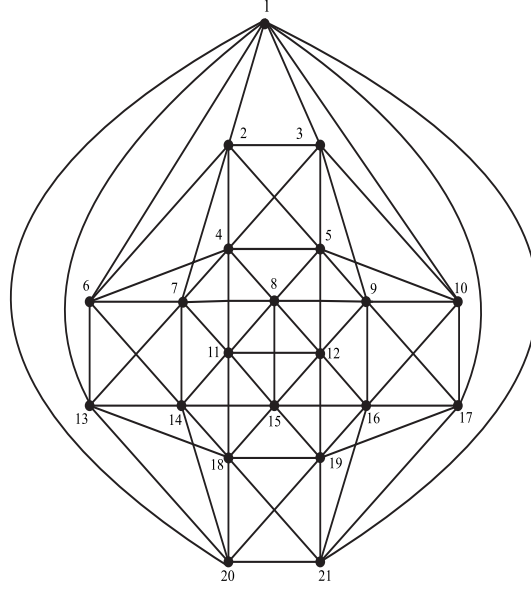

Fig. 7. A 5-factor-critical 1-planar graph.

For Figure 7 we only change the given values of three variables  $N$ ,  $D$  and  $EN$  in program “factor\_critical.cpp” as follows. In this program the input data - adjacency list is still file “graph\_6.txt”. To run directly it we only rename the input data-adjacency list “graph\_7.txt” of the present graph as “graph\_6.txt”. Then run “factor\_critical.cpp”, and the results are stored in “factor.txt”.

```

1 #define N 21 //N is the vertex number of the graph
2 #define D 8 //D is the maximum degree of the graph
3 #define EN 5 //EN is the number of vertices arbitrarily deleted in the
graph

```

For Figure 8(a) we only change the given values of three variables  $N$ ,  $D$  and  $EN$  in program “factor\_critical.cpp” as follows, and rename the input data - adjacency list “graph\_8(a).txt” as “graph\_6.txt”. Then run “factor\_critical.cpp”, and the results are in “factor.txt”.

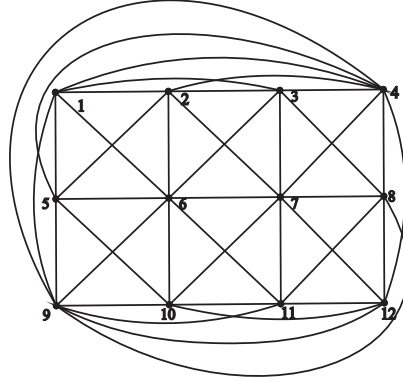

Fig. 8 (a). A 4-factor-critical optimal 1-planar graph.

For Figure 8(b) we only change the given values of three variables  $N$ ,  $D$  and  $EN$  in program “factor\_critical.cpp” as follows, and change the input data - adjacency list’s name “graph\_8(a).txt” as “graph\_6.txt”. Then run “factor\_critical.cpp”, and the results are in “factor.txt”.

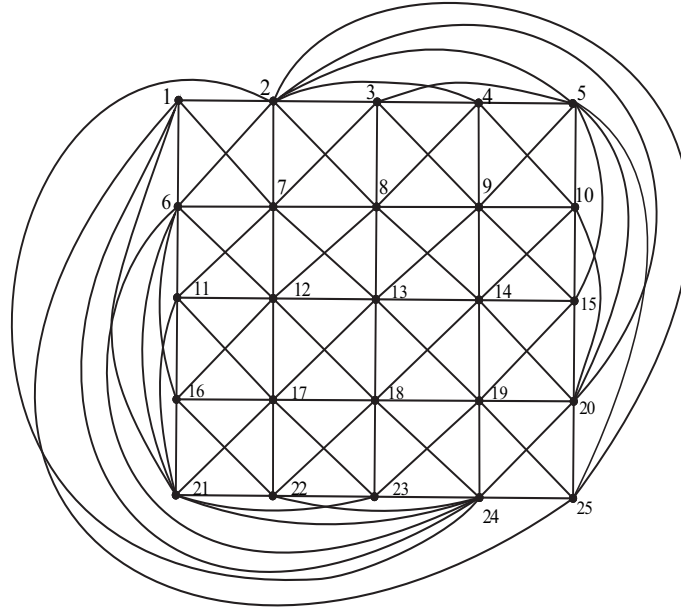

Fig. 8 (b). A 5-factor-critical optimal 1-planar graph.

```

1 #define N 25 //N is the vertex number of the graph
2 #define D 10 //D is the maximum degree of the graph
3 #define EN 5 //EN is the number of vertices arbitrarily deleted in the
graph

```
